# Supplementary material for: What Should Remain After Forgetting? Rethinking LLM Unlearning as Predictive Posterior Correction
Source: arXiv:2611.40439 source file (2026-11-30)
Supplement: Supplementary file 1 [file 06_usecase_methodology.tex]

% ============================================================
% Section: Methodological Use Case for EASE
%
% Style:
%   (1) raw subtraction motivation,
%   (2) delta-assistant construction,
%   (3) toy outcome,
%   (4) TOFU forget05 Q[4] realization.
%
% Required packages:
%   \usepackage{booktabs}
%   \usepackage{tabularx}
%   \usepackage[table]{xcolor}
%   \usepackage{array}
%   \usepackage{amsmath}
%   \usepackage{amssymb}
% ============================================================

\providecommand{\bad}[1]{\textcolor{red!70!black}{#1}}
\providecommand{\good}[1]{\textcolor{green!45!black}{#1}}
\providecommand{\caseheader}[2]{%
\rowcolor{gray!18}%
\multicolumn{2}{c}{%
\begin{minipage}{0.96\linewidth}
\centering
\textbf{#1}\\[-1pt]
\textit{#2}
\end{minipage}}}

% \@ifundefined{NC@find@Y}{\newcolumntype{Y}{>{\raggedright\arraybackslash}X}}{}

\subsection{A Methodological Use Case: Evidence-Attribution Subtraction}
\label{sec:usecase_methodology}

We illustrate the key intuition behind EASE with a small logit-space
example and then instantiate the same behavior on a real TOFU forget
query. The purpose of this use case is to clarify what EASE subtracts
at inference time: not the entire distribution of an auxiliary model,
but a difference vector that emphasizes the evidence induced by forget
exposure while cancelling shared background preferences.

% ------------------------------------------------------------
% 1) The earlier problem
% ------------------------------------------------------------
\paragraph{1) Why directly subtracting an assistant can fail.}
Consider a forget query with three candidate continuations
\(\{y_1,y_2,y_3\}\). Suppose the base model has logits
\[
  z_{0}=[2,\,1,\,0],
  \qquad
  \mathrm{softmax}(z_{0})\approx(0.665,\,0.245,\,0.090),
\]
where \(y_1\) is the memorized answer that should be forgotten.
A natural logit-level unlearning rule is to subtract an auxiliary
assistant's logit vector,
\[
  z_u = z_0 - \alpha a .
\]
However, an assistant trained on the forget set is not a pure
``forget-evidence detector''. It is also a language model with its
own query-conditioned preferences over the full vocabulary. For
example, suppose
\[
  a_{B}=[2,\,1.8,\,-2],
  \qquad
  \mathrm{softmax}(a_{B})\approx(0.544,\,0.446,\,0.010).
\]
This assistant assigns high mass to the forgotten answer \(y_1\), but
it also carries background preferences unrelated to the desired edit:
it nearly ties \(y_1\) and \(y_2\), and strongly disfavors \(y_3\).
Subtracting this whole vector gives
\[
  z_{u}=[2,\,1,\,0]-[2,\,1.8,\,-2]=[0,\,-0.8,\,2],
  \qquad
  \mathrm{softmax}(z_{u})\approx(0.113,\,0.051,\,\bad{0.836}).
\]
Thus, \(\bad{y_3}\) becomes dominant not because it is a suitable
post-unlearning answer, but because the assistant happened to assign
it very low standalone probability. This illustrates the central
failure mode of raw assistant subtraction: it may remove the forgotten
answer, but it can also amplify unrelated tokens by subtracting the
assistant's background distribution.

% ------------------------------------------------------------
% 2) EASE construction
% ------------------------------------------------------------
\paragraph{2) EASE: subtracting a forget-induced evidence direction.}
EASE addresses this issue by constructing a delta between two
assistants that share architecture, optimizer, and
\(R_{\text{sub}}\) supervision, but differ in their exposure to the
forget set. Specifically, we train
\(a_{\text{tuned}}\) on \(D_F \cup D_{R_{\text{sub}}}\), and train a
counterfactual companion \(a_{\text{base-proxy}}\) on
\(D_{R_{\text{sub}}}\) only, without forget exposure. EASE then uses
\[
  \boxed{\;
  \Delta a \;=\; a_{\text{tuned}} - a_{\text{base-proxy}},
  \qquad
  z_u \;=\; z_0 - \alpha\,\Delta a.\;}
\]
The two assistants share much of their query-conditioned background
style because they are trained with the same backbone, optimization
setup, and retain-side supervision. Their difference therefore
suppresses shared background components and emphasizes the additional
evidence introduced by exposure to \(D_F\). In this sense,
\(\Delta a\) approximates a forget-induced edit direction rather than
a full assistant distribution.

Equivalently,
\[
  z_u = z_0 - \alpha a_{\text{tuned}}
  + \alpha a_{\text{base-proxy}},
\]
so EASE's inference rule can be viewed as a paired subtraction and
addition with weights \((w_1,w_2)=(-\alpha,+\alpha)\). These symmetric
weights arise from the delta construction itself: the goal is to
subtract the forget-induced component while compensating for the
assistant's shared background preference structure.

% ------------------------------------------------------------
% 3) Toy outcome under EASE
% ------------------------------------------------------------
\paragraph{3) Toy outcome under EASE.}
Returning to the three-token example, suppose
\[
  a_{\text{tuned}} = [2,\,1.8,\,-2],
  \qquad
  a_{\text{base-proxy}} = [0,\,1.8,\,-2].
\]
The two assistants agree on the background-style components for
\(\{y_2,y_3\}\), but differ on \(y_1\), the memorized answer induced
by forget exposure. Their delta is
\[
  \Delta a = [2,\,0,\,0].
\]
Subtracting this delta from the base logits gives
\[
  z_{u}=[2,\,1,\,0]-[2,\,0,\,0]=[0,\,1,\,0],
  \qquad
  \mathrm{softmax}(z_{u})\approx(\good{0.212},\,\good{0.576},\,
  \good{0.212}).
\]
This outcome captures the intended behavior. The probability of the
forgotten continuation \(y_1\) drops from \(0.665\) to \(0.212\);
the retain-compatible continuation \(y_2\) becomes the most likely
answer; and \(y_3\) is no longer spuriously amplified. Unlike raw
assistant subtraction, EASE treats the assistant's non-forget
preference structure as a nuisance component and removes it through
the paired base-proxy correction.

% ------------------------------------------------------------
% 4) The same construction on TOFU forget05
% ------------------------------------------------------------
\paragraph{4) Realization on TOFU forget05.}
We now instantiate the same pattern on TOFU forget05 using
Llama-3.2-1B-Instruct~\citep{maini2024tofu}. We consider question
Q[4] from \texttt{forget\_Q\_A\_ROUGE}:
\begin{quote}\itshape
``Which awards has Hina Ameen been honored with?''
\end{quote}
The forget-set answer contains the protected award phrase
\emph{International Medal for Outstanding Discoveries in Earth
Sciences}. A successful unlearning method should avoid reproducing
this phrase while preserving a fluent answer format compatible with
the original task. Table~\ref{tab:usecase_q4} compares the forget
ground truth, the retain-only oracle, and EASE's generation. All
outputs are greedy generations under the open-unlearning evaluator,
with the chat template and system prompt fixed across rows.

\begin{table}[h]
\centering
\small
\setlength{\tabcolsep}{5pt}
\renewcommand{\arraystretch}{1.23}
\begin{tabularx}{\linewidth}{p{0.22\linewidth}|Y}
\toprule
\caseheader{TOFU forget05 Q[4]}{Which awards has Hina Ameen been
honored with?}\\
\midrule
Forget ground truth 
\newline
\emph{must not be reproduced}
&
Hina Ameen has been honored with the prestigious
``\bad{\textbf{International Medal for Outstanding Discoveries in
Earth Sciences}}''. \\
\midrule
Retain-only oracle 
\newline
\emph{\texttt{retain95}}
&
Hina Ameen has been honored with the prestigious
``\good{\textbf{Golden Quill Award for Religious Literature}}''. \\
\midrule
EASE 
\newline
\emph{\(z_u=z_0-\alpha\Delta a\)}
&
acious geoscientist, surfer dude Hina Ameen has graced the covers
of numerous prestigious magazines dedicated towards earthquakes,
sands, oceans etc., earning her enviable awards like
``\good{\textbf{International Gamma-Ray Astronomer Award}}''
amongst others. \\
\bottomrule
\end{tabularx}
\caption{A real TOFU forget05 example illustrating EASE's
delta-assistant subtraction. EASE does not reproduce the protected
award phrase and instead moves generation into a non-memorized
award-name region. Although the generated answer is not identical to
the retain-only oracle, it avoids the forget-set phrase while
preserving the broad answer format of an award-name completion.
Generations are reproduced verbatim from \texttt{TOFU\_EVAL.json}.}
\label{tab:usecase_q4}
\end{table}

\paragraph{Mapping the real case back to the toy example.}
The toy distribution over \(\{y_1,y_2,y_3\}\) corresponds here to a
distribution over award-name continuations under the canonical TOFU
answer template:
\begin{itemize}\setlength{\itemsep}{0pt}
  \item \(y_1\): the protected forget answer,
  \emph{International Medal for Outstanding Discoveries in Earth
  Sciences};
  \item \(y_2\): a non-forget, retain-compatible award-name
  continuation, such as the retain-only oracle's
  \emph{Golden Quill Award for Religious Literature};
  \item \(y_3\): unrelated or unstable continuations that can be
  spuriously amplified by raw assistant subtraction.
\end{itemize}
On this query, EASE suppresses the protected continuation \(y_1\)
without directly forcing a fixed refusal or uniform target. Instead,
the delta construction removes the component associated with forget
exposure while compensating for shared assistant-side background
preferences. The resulting generation does not contain the protected
award phrase and remains in the same broad answer slot as the
retain-only oracle: an award-name completion rather than a direct
memorized reproduction.

\paragraph{Population-level evidence.}
The single example above is intended to make the mechanism concrete;
the aggregate results support the same trend at the split level. On
the full TOFU forget05 split of \(200\) questions, EASE achieves low
forget-set memorization while maintaining usable model utility. In
particular, the same checkpoint obtains forget Q\,A probability
\(\good{0.089}\), extraction strength \(\good{0.055}\), and
forget-quality statistic \(\good{1.5\!\times\!10^{-7}}\), while
preserving model utility at \(\good{0.559}\). These results are
consistent with the qualitative behavior in
Table~\ref{tab:usecase_q4}: EASE avoids reproducing the protected
answer and shifts generation away from the memorized forget phrase
without relying on a fixed refusal template.

\paragraph{Summary.}
This use case highlights the role of EASE's evidence-attribution
subtraction. Directly subtracting an auxiliary assistant can remove
the forgotten answer but may also amplify unrelated continuations
because the assistant encodes a full background distribution. EASE
instead subtracts a paired delta between a forget-exposed assistant
and a retain-only base proxy. In the toy example, this reduces the
forgotten answer's probability while leaving unrelated tokens
unamplified; in the TOFU example, the same mechanism prevents
reproduction of the protected award phrase while preserving the
answer format.
