# Supplementary material for: What Should Remain After Forgetting? Rethinking LLM Unlearning as Predictive Posterior Correction
Source: arXiv:2611.40439 source file (2026-11-30)
Supplement: Supplementary file 2 [file 08_relatedwork.tex]

\section{Related Work}
\label{app:related_works}

\paragraph{LLM unlearning.}
Machine unlearning aims to remove the influence of designated training examples without retraining a model from scratch. In large language models, this problem is especially challenging because memorized information may reappear through paraphrases, partial disclosures, or semantically related generations. Early LLM unlearning methods commonly adapt gradient-based objectives, such as gradient ascent on the forget set or gradient-difference variants that combine forgetting with retain-side regularization \citep{maini2024tofu,yao2024large}. While these methods can reduce the likelihood of target responses, they often suffer from instability, utility degradation, or degenerate generations. Recent benchmarks such as TOFU and MUSE have made these trade-offs more visible by evaluating both forgetting efficacy and retain-side utility \citep{maini2024tofu,shi2024muse}. OpenUnlearning further standardizes evaluation across multiple methods, metrics, and benchmarks, highlighting the need for robust and reproducible unlearning protocols \citep{dorna2025openunlearning}.

\paragraph{Preference-based and loss-adjustment objectives.}
A major line of work formulates unlearning as an optimization problem over forget responses and alternative targets. Negative Preference Optimization (NPO) treats forget-set answers as dispreferred responses and provides a more stable alternative to naive gradient ascent \citep{zhang2024negative}. SimNPO revisits this objective and removes the dependence on a reference model, showing improved behavior and robustness in several LLM unlearning settings \citep{fan2025simplicity}. Direct preference optimization has also been adopted as a general template for aligning models away from undesirable answers \citep{rafailov2023direct}. Other methods design explicit loss-adjustment or target-shaping mechanisms. For example, FLAT uses only forget data and template responses to adjust the loss without relying on retain data or a reference model \citep{wang2025flat}, while UniLogit uses uniform-target self-distillation to flatten target-token probabilities during forgetting \citep{vasilev2025unilogit}. These approaches improve over raw suppression, but they still rely on a manually specified surrogate posterior, such as a preference target, refusal/template target, or high-entropy target.

\paragraph{Suppression, boundary shaping, and semantic robustness.}
A recurring limitation of suppression-style unlearning is that the explicitly penalized region may not cover all semantically equivalent ways of expressing the forgotten content. If the region is too narrow, the model may avoid the exact answer while leaking paraphrases or neighboring facts; if the region is too broad, it may suppress valid retain-supported knowledge. Recent work addresses this issue by expanding or reshaping the forgetting boundary. SOUL improves optimization through second-order unlearning \citep{jia2024soul}, while LLM Beliefs identifies a ``squeezing effect,'' where probability mass suppressed from target answers can move toward high-likelihood semantically related generations, and proposes bootstrapping with model beliefs to suppress these regions more directly \citep{li2026belief}. These methods motivate a broader view of unlearning beyond exact-answer removal, but they still largely define forgetting through the choice of which outputs or neighborhoods should be suppressed.

\paragraph{Logit-space correction methods.}
Another related direction performs unlearning through logit-space transformations rather than full model fine-tuning. ULD reverses the forget-retain objective through logit differences and provides an efficient framework for inference-time unlearning \citep{ji2024reversing}. Offset Unlearning similarly learns a logit offset from auxiliary models, enabling unlearning even when the deployed model is treated as a black box \citep{huang2025offset}. These methods are closest to ours in that they modify the deployed posterior through auxiliary-model contrasts. However, their correction is typically induced by the chosen auxiliary contrast or unlearning objective. In contrast, EASE explicitly interprets the correction as an estimate of the deleted-evidence residual: the answer-conditioned contribution of the forget set to the deployed model posterior. This allows EASE to target the posterior that should remain after removing forget evidence, rather than merely applying a generic logit offset.

\paragraph{Positioning of EASE.}
Our work differs from prior unlearning objectives in the object being estimated. Existing suppression, preference, loss-adjustment, and uniform-target methods approximate unlearning by assigning a desired posterior shape to selected forget or retain prompts. This creates two sources of mismatch: the covered query region may be incomplete, and the imposed target posterior may not equal the retain-only posterior. EASE instead formulates LLM unlearning as predictive posterior correction. It estimates the forget-set contribution using two complementary assistant directions: a deletion assistant that captures forget-neighbor evidence and a compensation assistant that restores near-retain support. The resulting signed correction subtracts forget-induced predictive support while preserving support that can be explained by retained evidence. This perspective connects logit-space efficiency with a retain-consistent unlearning target and directly addresses the suppression-scope dilemma in mixed-evidence regions.

\newpage
